# Supplementary material for: Revealing the band structure of ZrTe$_5$ using Multicarrier Transport
Source: arXiv:2209.06797 ancillary file (2023-01-19)
Supplement: Supplementary file 1 [file Supporting_Information.pdf]

# Supporting Information: Revealing the band structure of $ZrTe_5$ using Multicarrier Transport

Zoltán Kovács-Krausz,[1,2] Endre Tóvári,[1,3,*] Dániel Nagy,[4] Albin Márffy,[1,2] Bogdan Karpiak,[5] Zoltán Tajkov,[6] László Oroszlány,[4,7] János Koltai,[8] Péter Nemes-Incze,[6] Saroj Dash,[5] Péter Makk,[1,3] and Szabolcs Csonka[1,2]

[1]*Department of Physics, Institute of Physics, Budapest University of Technology and Economics, Műegyetem rkp. 3., H-1111 Budapest, Hungary*

[2]*MTA-BME Superconducting Nanoelectronics Momentum Research Group, Műegyetem rkp. 3., H-1111 Budapest, Hungary*

[3]*MTA-BME Correlated van der Waals Structures Momentum Research Group, Műegyetem rkp. 3., H-1111 Budapest, Hungary*

[4]*Department of Physics of Complex Systems, ELTE Eötvös Loránd University, 1117 Budapest, Hungary*

[5]*Department of Microtechnology and Nanoscience, Chalmers University of Technology, SE-41296, Göteborg, Sweden*

[6]*Centre for Energy Research, Institute of Technical Physics and Materials Science, 1121 Budapest, Hungary*

[7]*MTA-BME Lendület Topology and Correlation Research Group, Budapest University of Technology and Economics, 1521 Budapest, Hungary*

[8]*ELTE Eötvös Loránd University, Department of Biological Physics, 1117 Budapest, Hungary*

## I. DEVICE FABRICATION, TRANSPORT MEASUREMENTS AND MULTICARRIER FITS

The CVT-grown $ZrTe_5$ samples were obtained from HQ Graphene. Thin crystals were produced via exfoliation of the macroscopic crystals. The adhesive tape method was used, starting from a macroscopic $ZrTe_5$ sample and using semiconductor dicing tape to cleave the crystal, before pressing the tape to a $SiO_2$ substrate (approx. 290 nm thick). During exfoliation, the $ZrTe_5$ favorably cleaves into regular rectangular single crystals of several μm dimensions, where the longer edge of the crystal is parallel to the major crystallographic axis running along the Zr atom chains. Crystals of thickness between 50-150 nm (verified by atomic force microscopy) were selected for device fabrication. Metallic contacts were created on selected crystals using electron beam vapor deposition. A Cr adhesion layer of 10 nm was deposited, before a main layer of 80-110 nm Au. To prepare a cleaner surface on the $ZrTe_5$, an Ar ion beam milling step was performed immediately before metal deposition under vacuum. A high angle of incidence for the ions was used, with an Ar gas flow rate of 10 sccm, resulting in a 1.5 mTorr chamber pressure; exposure was 60 seconds at 60 W of power.

For each regular rectangular device, two larger metallic contacts at the ends along the longitudinal direction (x-axis) were used for passing bias current, and several side contacts were created to measure longitudinal ($\rho_{\mathrm{xx}}$) resistivity in a four-terminal configuration as well as transverse ($\rho_{\mathrm{xy}}$) resistivity. The devices were cooled down in a variable temperature insert (VTI) of a helium cryostat with an 8T superconducting magnet, with $B_{\mathrm{z}}$ field configuration. During measurement, low frequency AC bias voltage (between 100-500 μV) was applied along the x-axis of the devices, measuring the bias current back with a lock-in amplifier. At each temperature point between 1.5-305 K, the $B_{\mathrm{z}}$ field was swept while simultaneously recording the $\rho_{\mathrm{xx}}$ and $\rho_{\mathrm{xy}}$ values.

To process the experimental data, a symmetrization (antisymmetrization) of the $\rho_{\mathrm{xx}}$ ($\rho_{\mathrm{xy}}$) signals was performed. For this, first we interpolated the raw data in order to get evenly spaced data points in $\pm B$ pairs; even and odd curves were generated using $\rho_{\mathrm{xx}}(B) = 1/2 \times (\rho_{\mathrm{xx}}(B) + \rho_{\mathrm{xx}}(-B))$ and $\rho_{\mathrm{xy}}(B) = 1/2 \times (\rho_{\mathrm{xy}}(B) - \rho_{\mathrm{xy}}(-B))$. We note that, thanks to the regular contact geometry, the raw curves themselves were usually close to symmetric/antisymmetric.

Apart from the device (hereafter designated D1) presented in the main text (transport measurements in Fig. 2), the same measurements on four similar devices designated D2-D5 are presented in Fig. S1. The upper row contains the $\rho_{\mathrm{xy}}$ data while the middle row the $\rho_{\mathrm{xx}}$ data. The temperature dependence of $\rho_{\mathrm{xx}}$ without applied field, for determining $T_{\mathrm{p}}$, is shown in the third row of the figure.

The overall temperature-based behavior is consistent between the different devices. At the lowest temperatures, the Shubnikov-de Haas oscillations (SdHO) features in $\rho_{\mathrm{xx}}$ are always present, but the overall apparent slope of the $\rho_{\mathrm{xy}}$ curves at high fields changes from device to device. In addition, while the magnitudes of the transverse magnetoresistivites $\rho_{\mathrm{xy}}$ are consistent between all devices D1-D5, the longitudinal resistivity $\rho_{\mathrm{xx}}$ varies by almost an order of magnitude. In the figure the devices D2-D5 have been arranged in order of increasing resistivity, and the resistivity of D1 falls in the middle. Importantly, the results of the MCT fitting method, which show the contributions of different charge carriers from $i = 1$ to $i = 5$ in the MCT model are remarkably similar for all devices. This can

* tovari.endre@ttk.bme.hu

be seen in Fig. S2. The overall fitting method for obtaining the $\sigma_i$ and $\mu_i$ values is the same as described in the main text, while additional details for the method are described further below. The MCT characteristics of device D1 in the main text appear identically in the other devices: the necessity for an edge-confined carrier with no field dependence ($i = 1$ with $\mu_1 = 0$), the necessity of using NC=5 near $T_p$, the mobility trends with temperature without significant jumps, and the temperature-dependent depletion of carriers resulting in NC=4 and even NC=3 at high and low temperatures.

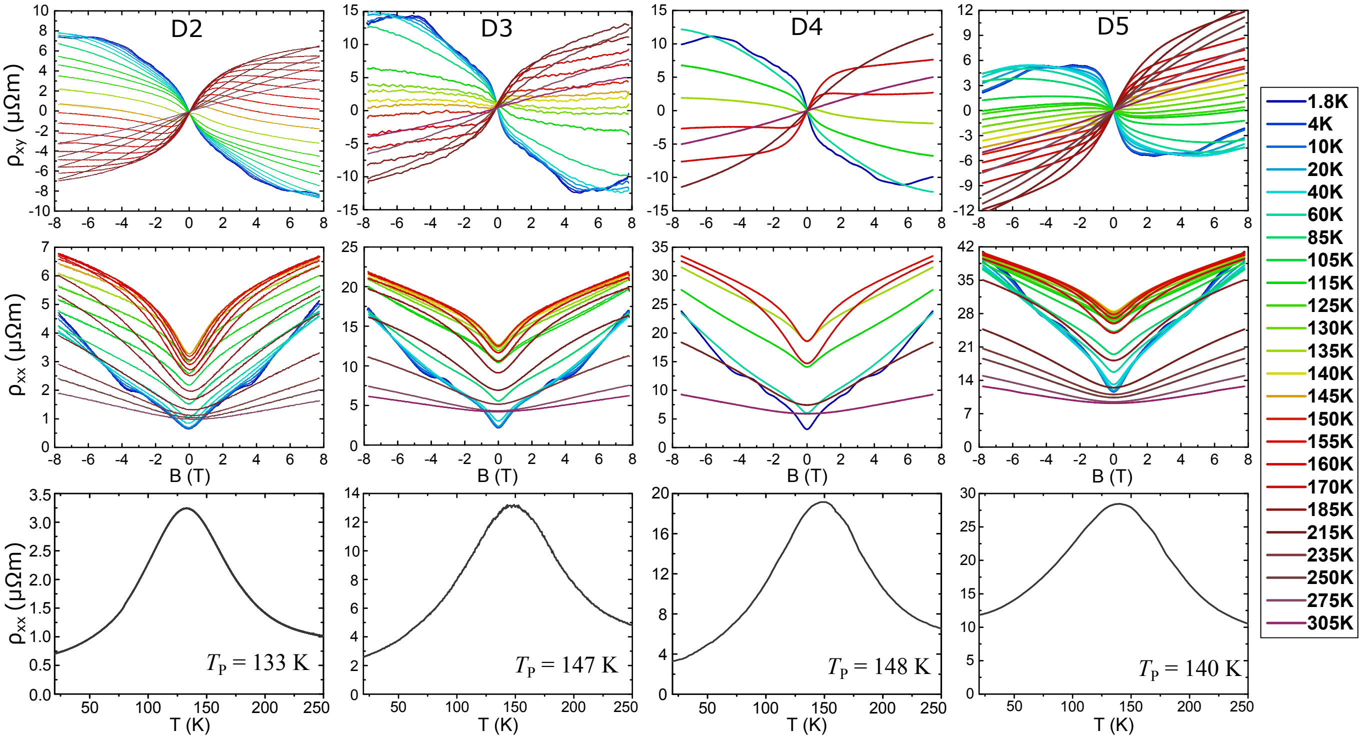


Figure S1. Transverse (first row) and longitudinal (middle row) resistivity data for devices D2-D5. The characteristic peaks $T_p$ are shown in the zero-field temperature dependence curves in the last row.

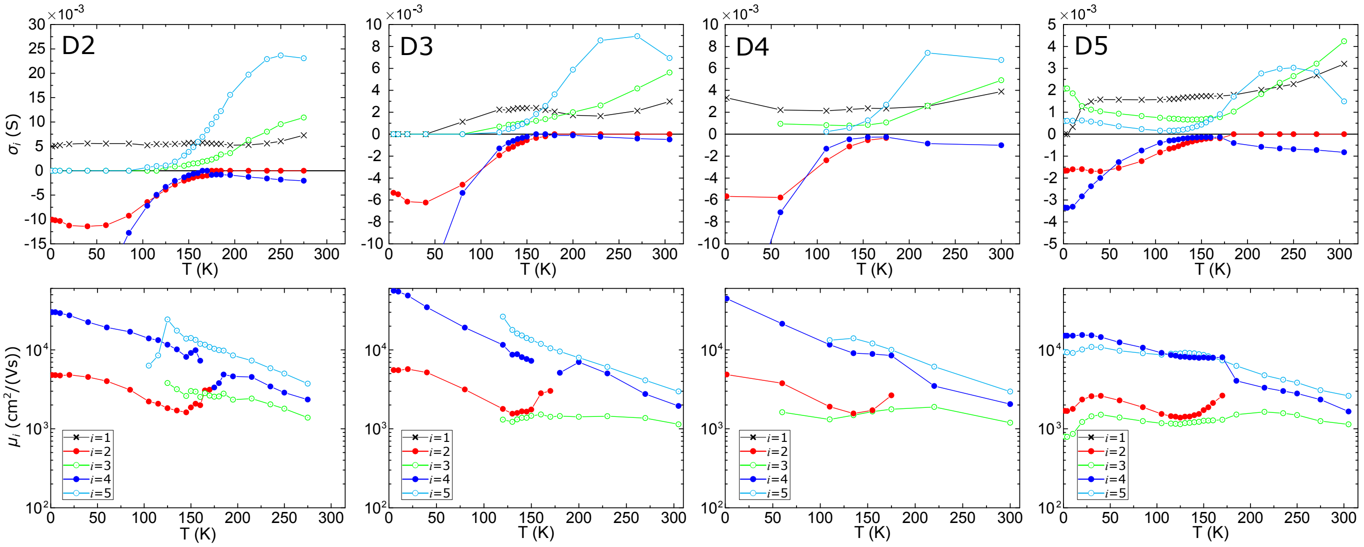


Figure S2. Fitting results of the MCT model for devices D2-D5. The black ($i = 1$) carrier is the field-independent edge-confined carrier. A total of five carriers (NC=5) is required near $T_\mathrm{p}$, while NC=4 is adequate further from it, and even NC=3 at very low temperatures.

## II. SHUBNIKOV-DE HAAS OSCILLATIONS

Oscillations measured at a temperature of 1.5 K are presented for devices D1 (dark cyan) and D3 (dark red) in Fig. S3 (a), plotted as function of inverse field $B^{-1}$. The oscillations in $\rho_\mathrm{xx}$ are plotted after smoothing and subtracting a background via fitting a polynomial (3rd order) and gaussian to the $\rho_\mathrm{xx}(B)$ data. The high-field amplitude of the signal is larger in case of device D1 compared to D3, while oscillations at lower fields are comparable. However, oscillations corresponding to Landau levels $N = 2$ to $N = 7$ can be found in both devices ($N = 1$ is not visible due to upper magnetic field limitations of the measurement). The oscillation frequency of the SdHO, $B_\mathrm{F}$, which relates to the Fermi surface cross section perpendicular to the measurement field $B_\mathrm{z}$, can be obtained using the fast Fourier transform (FFT), or from the slope of the Landau level index plotted as function of inverse magnetic field (Landau fan diagram). Fig. S3 (b) shows the FFT of both oscillations. For device D3, the FFT shows two distinct peaks revealing two frequencies in the SdHO, at approximately 4.4 and 5.5 T respectively. In contrast, device D1 shows a widened peak of 5.2 T with a shoulder at 6.2 T. The two distinct frequencies in both devices are more readily apparent in the Landau fan diagrams in Fig. S3 (c) (device D1) and (d) (device D3).

We have plotted both the maxima (filled circles) and minima (empty squares) as a function of inverse field. In both cases, at a field of around 1.7 T, the slope of the datapoints visibly changes, while remaining close to linear above and below. Like the two peaks in the FFT, this suggests the coexistence of two oscillations in the SdHO, with one being more dominant at high fields. We have fitted each section of the fan plots with its own linear equation, obtaining the slope (corresponding to the frequency $B_\mathrm{F}$) and intercept $\gamma$, which relates to the Berry phase $\Phi_\mathrm{B}$ by $\gamma = \frac{1}{2} - \frac{\Phi_\mathrm{B}}{2\pi} - \delta$. Thus, in 2D systems for a trivial Berry phase we expect half-integer $\gamma$, and for non-trivial, an integer $\gamma$ ($\delta$=0); while in case of a 3D system the additional phase shift $\delta$ is $\pm 1/8$ [1]. We can see that the linear fits to the fan plots for fields below 1.7 T (blue) result in an intercept $\gamma \approx 1 + 1/8$ for both devices, consistent with a 3D Dirac band. The fits above 1.7 T (red) have $\gamma$ closer to 1/2, suggesting the additional contribution of another (trivial) electron pocket.

The Landau fan diagram fits are consistent with the results of the MCT model, which also suggest the coexistence of two reasonably high mobility electron carriers at low temperature. During the MCT analysis we have associated the higher mobility carrier with the Dirac-like electron band ($i = 4$, blue). However, the lower mobility ($i = 2$, red) carrier of the MCT model cannot be associated with any single electron side-pocket, as there are multiple relevant pockets in the band structure. It is possible that the trivial component of the oscillation is caused by one of these pockets, and the lower mobility and higher effective mass results in its SdHO contribution being stronger at larger fields, and negligible at smaller fields.

The oscillation frequency $B_\mathrm{F}$ can be used to obtain the Fermi surface cross sectional area in the xy-plane. The Dirac-like electron pocket at $\Gamma$ maintains a reasonably circular cross section perpendicular to $k_\mathrm{z}$, in both ARPES results such as Ref. [2] as well as our DFT results. Using the oscillation frequency, the cross section can be expressed by $S_\mathrm{F} = \frac{2e\pi}{\hbar} B_\mathrm{F}$, resulting in $S_\mathrm{F,D1} = 4.56 \times 10^{-4} \mathring{A}^{-2}$ and $S_\mathrm{F,D3} = 4.04 \times 10^{-4} \mathring{A}^{-2}$. Assuming a circular in-plane

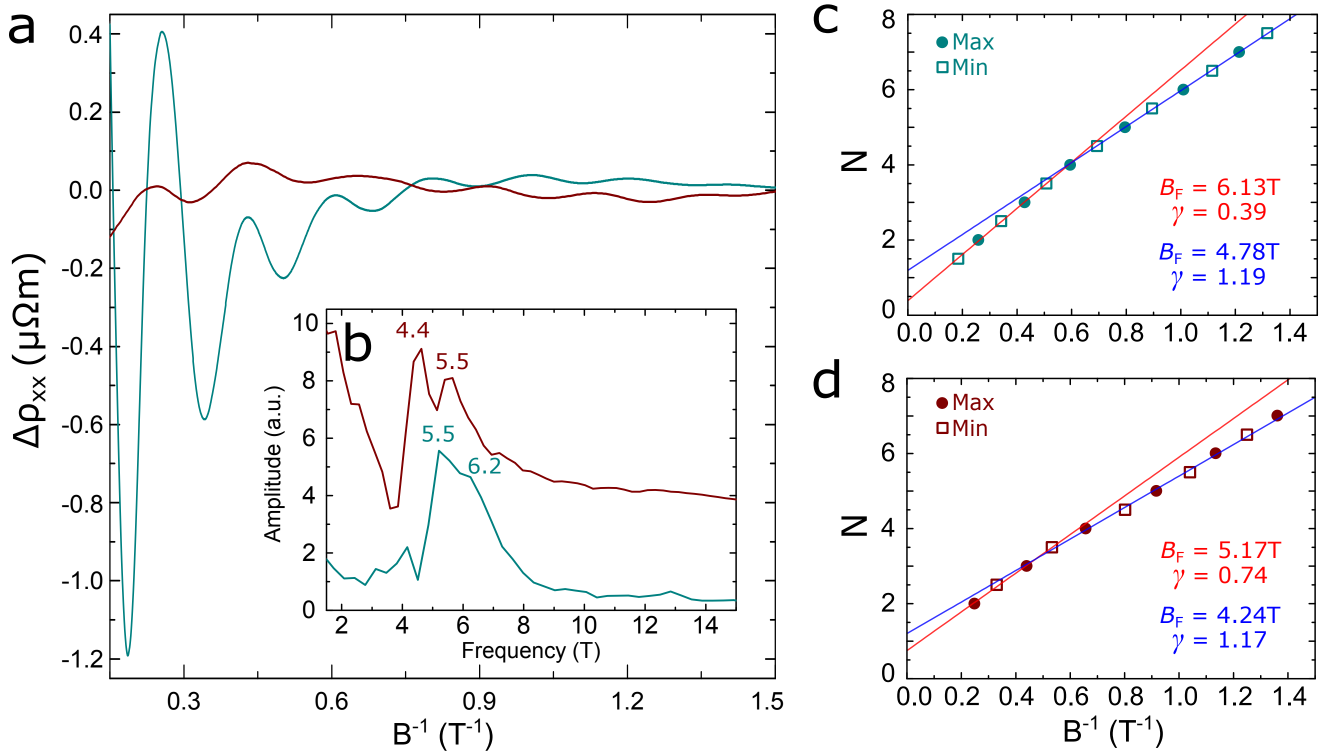


Figure S3. Shubnikov-de Haas oscillations measured in devices D1 (dark cyan) and D3 (dark red). (a) Oscillations in $\rho_{\mathrm{xx}}$ after smoothing and background removal. (b) fast Fourier transforms of the data in (a), with approximate values of peak frequencies $B_{\mathrm{F}}$ highlighted. (c)(d) Landau fan diagram of D1 (c) and D3 (d). There are two distinct slopes in each case, corresponding to two distict frequencies in the oscillation. Linear fit slope ($B_{\mathrm{F}}$) and intercept ($\gamma$) are shown.

cross section we obtain $k_{\mathrm{F,xy}} \approx 1.1 - 1.2 \times 10^{-2} \mathring{A}^{-1}$. This value is comparable with the ARPES results at 2 K temperature of Ref. [2], of approximately $1.5 \times 10^{-2} \mathring{A}^{-1}$ for both $k_{\mathrm{F,x}}$ and $k_{\mathrm{F,y}}$, as well as with our DFT results at approximately 100 meV (accounting for the band shift at 2 K as well as some n-doping) of $k_{\mathrm{F,x}} = 1.15 \times 10^{-2} \mathring{A}^{-1}$ and $k_{\mathrm{F,y}} = 1.57 \times 10^{-2} \mathring{A}^{-1}$. This gives further support, along with the obtained intercept $\gamma$, that the oscillation observed at lower fields in the SdHO corresponds to the Dirac-like high mobility $i = 4$ electron band in our MCT model.

For the trivial electron side pocket, the band along $A_1$-T in the DFT also appears in the ARPES measurements of Ref. [2]. While measurements at 2 K for this band are not presented, by extrapolating the observed band shift linearly to 2 K we can estimate a similar $k_{\mathrm{F,xy}}$ on the order of $1 - 2 \times 10^{-2} \mathring{A}^{-1}$. This can be compared with the estimation from SdHO frequency of $k_{\mathrm{F,xy}} \approx 1.2 - 1.4 \times 10^{-2} \mathring{A}^{-1}$, indicating that the observed oscillation could be caused by this electron pocket.

## III. FITTING METHOD: DISCONTINUITIES AND THE EDGE-LOCALIZED CARRIER

As described in section III. of the main text, the fitting method uses an MCT approach with multiple independent carriers, each with its own carrier density, mobility, and sign, which leads to a particular magnetic field dependent contribution to $\sigma_{\mathrm{xx}}$ and $\sigma_{\mathrm{xy}}$. The inputs to the fitting procedure are the experimental $\sigma_{\mathrm{xx(xy)}}(B)$ curves, and a particular choice of NC for the model, for which we have used values between 2-6 (the extremal values of NC=2 and NC=6 did not end up reasonable at any temperatures for any devices; more on this further below). In addition, since there is a large number of fitting parameters, to avoid potential local minima, each fit (for each particular NC value) is repeated several (50-250) times using randomized starting parameters, and we use a histogram method to select the most frequent fit results as the final values, as long as the mean square error (MSE) is reasonably low. Fig. S4 demonstrates this on a set of 250 fits using NC=5 for the 140 K measurement curves of device D1. It can be seen that the vast majority of attempts fall into one particular bin, and this solution also has a significantly lower MSE than the majority of the remaining attempts that did not fall into the same bin (Fig. S4 (g)).

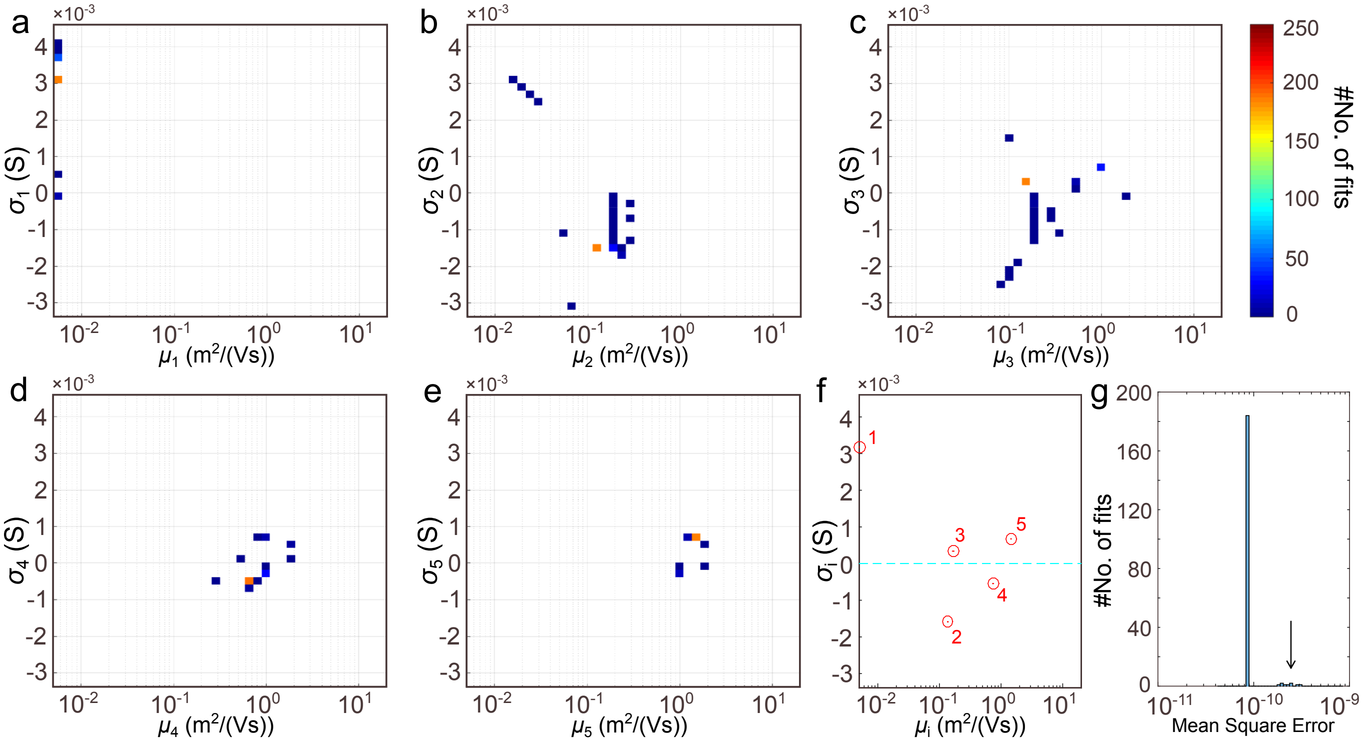


Figure S4. Histograms of 250 NC=5 fit attempts on device D1 at 140 K. (a-e) binned results of the converged $\sigma_{\mathrm{i}}$ and $\mu_{\mathrm{i}}$ parameters for each of the five carriers; the color represents the number of occurrences in each bin. The majority of the results are in one particular bin (orange). (f) The most frequent results of the five carrier parameters. (g) Histogram of the mean square error (MSE) of the fit attempts. For the results that do not fall into the most common bin, the MSE is usually worse, as highlighted by the arrow.

One of the main problems of initial fitting attempts was that, similar to other published works that use NC=2, we commonly observe large jumps in $\mu_{\mathrm{i}}$, up to two orders of magnitude, and simultaneous discontinuities in $\sigma_{\mathrm{i}}$ for the same carrier. This happens even at NC=6 as depicted in the top row of Fig. S5. Such jumps in mobility within a small temperature range are unreasonable, and are probably artifacts of an inadequate fitting procedure. In particular, we notice that these jumps often involve an unrealistically low mobility value well below 100 $\mathrm{cm}^2/\mathrm{Vs}$. Additionally, a carrier with unexpectedly low mobility is always present for all temperatures. Considering the $B$ field contribution of a carrier within the MCT model, a very low mobility corresponds to a behavior that is near-constant with field, having zero Hall contribution and some near-constant longitudinal contribution in the studied field range.

On the other hand, if we envision a transport band that is localized at the edges of the $\mathrm{ZrTe}_5$ device, it would result in a similar behavior in the transport measurement, lacking $B$ field dependence and having only a constant $\sigma_{\mathrm{xx}}$ contribution. Therefore, we model this edge-confined carrier, by fixing the mobility of one carrier at zero (by arbitrary choice $\mu_1 = 0$). As seen in the subsequent fitting results on the lower row of Fig. S5, the large jumps in mobility are

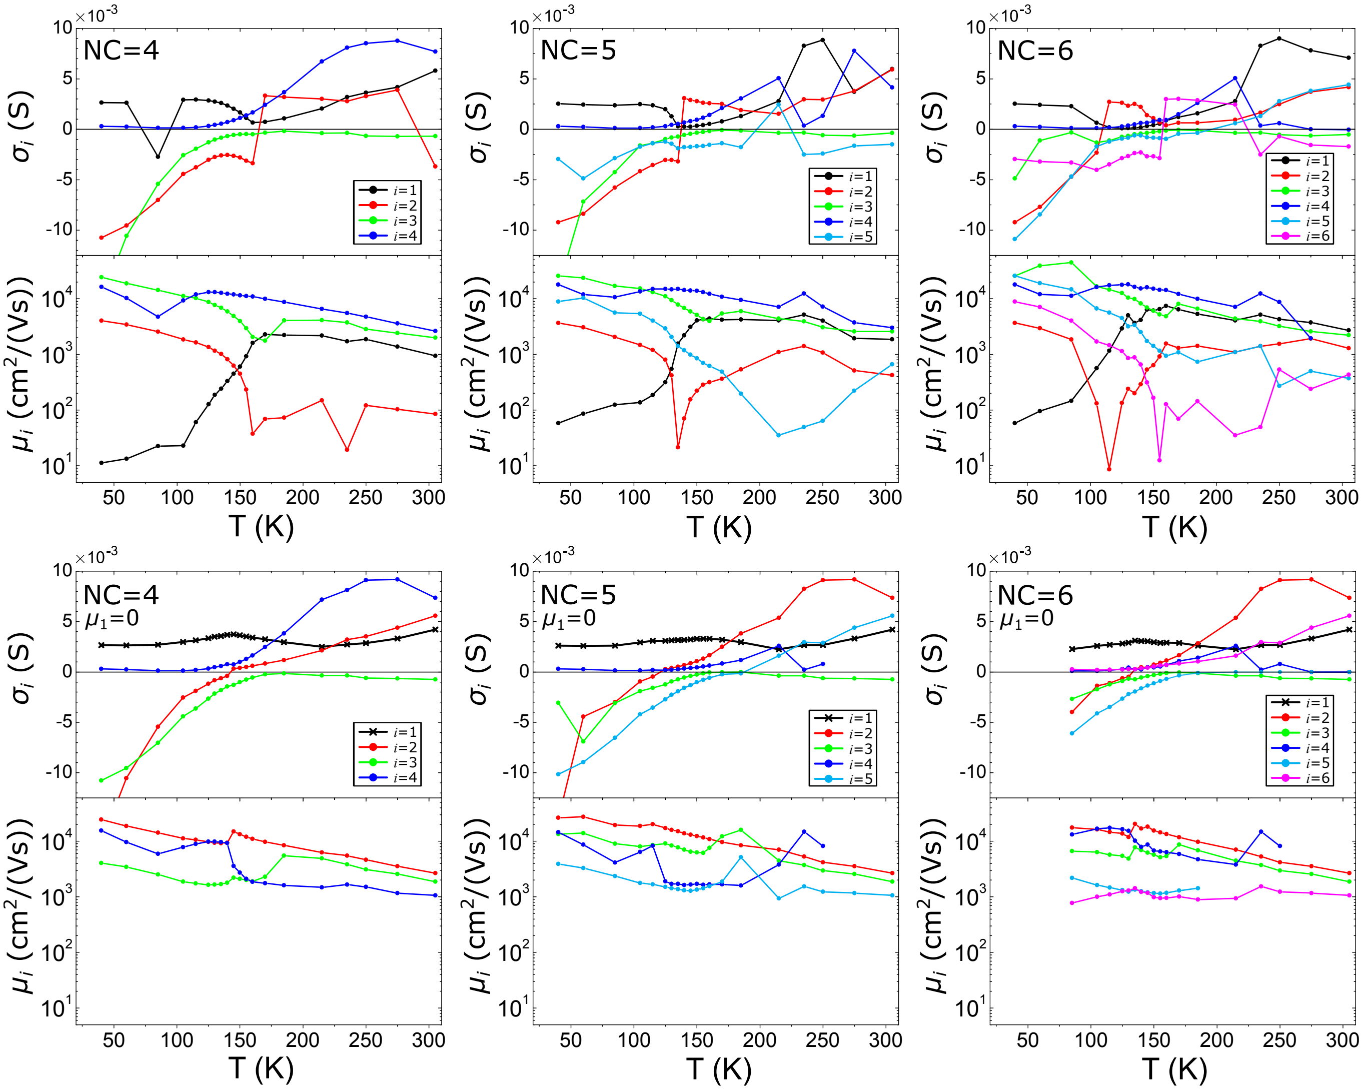


Figure S5. MCT fitting results for device D1 for different NC values. Top row: all carrier mobilities are free fitting parameters. Carrier mobilities reach unreasonably low values, corresponding to large jumps in $\sigma_\mathrm{i}$ and sign change. Bottom row: $\mu_1$ is fixed to zero, representing a field-independent conductivity contribution. $\sigma_1$ has little temperature dependence. The discontinuities are less pronounced and mobility curves are smoother. Resolving the remaining sign changes involves determining which NC value is appropriate at each temperature.

resolved in the same dataset and, for the most part, mobility evolution with temperature becomes smoother, even at different NC values. Here the black color represents the edge-localized carrier. Note however that, at this point, some smaller discontinuities in mobility as well as $\sigma_\mathrm{i}$ still remain, as well as an additional peculiarity that in some cases a carrier crosses the $\sigma_\mathrm{i} = 0$ line (changes sign). To resolve these, we must consider within the context of the MCT model that, as the temperature changes, the contribution of certain electron and hole bands may become vanishingly small, leading to an expectation of NC change at some temperatures.

## IV. FITTING METHOD: NC SELECTION AND ERROR ANALYSIS

During the fitting procedure, the $\sigma_\text{i}$ and $\mu_\text{i}$ (where $i \in [1, NC]$) results are obtained for each NC from 2 to 6 at each individual temperature. Following this, we determine the temperature-dependent behavior of each individual carrier in the MCT model using a few reasonable assumptions. First, within a small temperature range there should be no dramatic jump in either $\sigma_\text{i}$ nor $\mu_\text{i}$ for a particular carrier, such that the temperature trend remains relatively smooth. Second, in conditions where one carrier becomes negligible in $\sigma_\text{i}$ (for example, a hole type carrier freezing out at low temperature), the values for the remaining relevant carriers can be obtained by reducing NC (essentially removing the negligible carrier from the fit). Third, the signed $\sigma_\text{i}$ values should not cross zero for any particular carrier, since we treat electrons and holes separately.

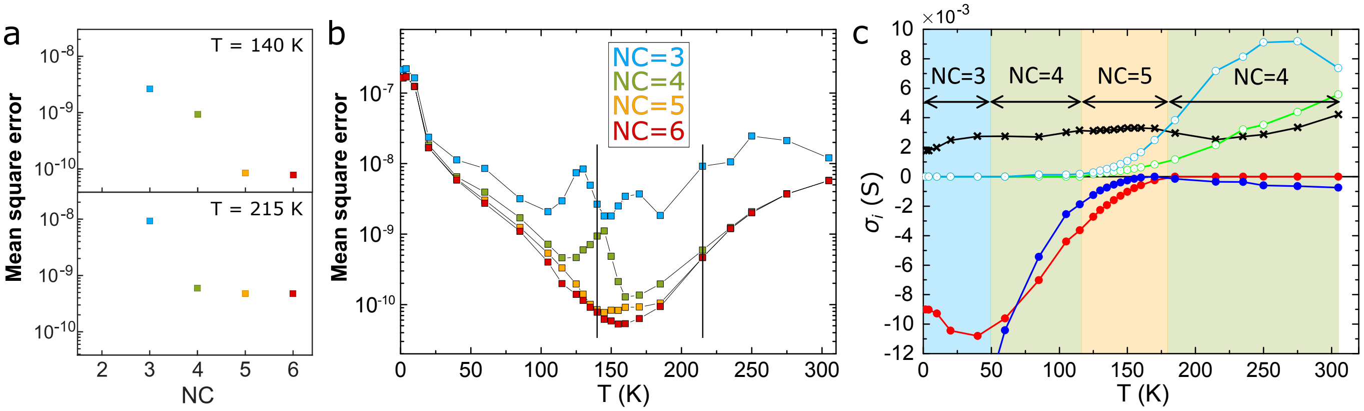


Figure S6. MSE analysis of MCT fits using different number of carriers. (a) MSE of NC=3 to NC=6 at 140 K and 215 K. MSE stops improving at NC=5 in the former and NC=4 in the latter case. (b) Temperature dependence of MSE of the fits. NC=6 and NC=5 do not differ significantly; NC=4 diverges from NC=5 near $T_\text{p}$, while at low temperatures NC=3 also becomes comparable to the others. Vertical lines correspond to the plots of (a). (c) The final MCT model result of $\sigma_\text{i}$ for device D1 based on MSE analysis. None of the carriers changes sign and there are no noticeable discontinuities with temperature.

The selection of the appropriate NC by temperature is not always straightforward. A lower bound can easily be determined by looking at whether the fit result actually follows the fitted data curve closely (as in Fig. 3 of main text). For example, we find that NC=2 is inadequate at any temperature for any device. On the other hand, if a particular value of NC leads to an appropriate fit, then increasing NC will also maintain an appropriate fit to the data curve. In Fig. S6 (a), the MSE value of the fits can be seen to decrease with increasing NC, up to a particular value. For the $T = 140$ K fits this occurs at NC=5 while further away from $T_\text{p}$, at 215 K, it occurs already at NC=4. Looking at the entire temperature range, the MSE evolution of each NC value can be seen in Fig. S6 (b). Here we notice that, for the most part, NC=5 and NC=6 are very close, while NC=4 only diverges from them in a temperature range near the $T_\text{p}$ of our $ZrTe_5$ devices. Meanwhile, the MSE of NC=3 maintains a higher value, but for very low temperature ranges the other MSE curves increase and become comparable with it. For the most part, selecting the smallest NC value at each temperature that does not yet lead to a noticeable increase in MSE, leads to a reasonable temperature dependence of the individual carriers. We have represented this on the final $\sigma_\text{i}$ values of device D1 in Fig. S6 (c): the temperatures where a carrier's contribution becomes negligible end up being the temperatures where the switch to a different NC value happens. The fact that the MSE analysis and expected change of best-fit NC value at a particular temperature coincides with one carrier's $\sigma_\text{i}$ contribution vanishing at the same temperature, offers support for the validity of the MCT model.

To further support the NC selection, we have investigated the individual relative errors of the $\sigma_\text{i}$ results at each NC. At temperatures where the the MSE values of two different NC are similar, the higher NC tends to result in larger uncertainties in the fit results. For example, the NC=4 errors jump to higher values at low temperatures, compared to NC=3. The NC=5 errors are the smallest of all near $T_\text{p}$. Meanwhile, increasing to NC=6 results in larger uncertainties across the range. In addition, the $\sigma_\text{i}$ and $\mu_\text{i}$ values in such cases often develop large jumps once again, or result in one or multiple carriers changing sign, which are not consistent with expectations of the MCT model. An additional observation is that, when going from NC=5 to NC=6 at a temperature where NC=5 is recommended by the MSE analysis, NC=6 results in almost exactly the same $\sigma_\text{i}$ and $\mu_\text{i}$ results, except for one carrier that becomes split into two new carriers with similar $\sigma_\text{i}$ and slightly different $\mu_\text{i}$. The values for these split carriers also show the noticeably larger errors in this case. In addition, the NC=6 fitting procedure commonly fails to converge below 85 K. As a

result of these considerations, we have not found NC=6 to be appropriate at any temperature. It does not offer an improvement in MSE over NC=5, and shows instabilities and carrier sign changes in the temperature trends. If additional electron pockets (as seen in band structure calculations) do in fact contribute to the transport behavior, it is likely that they have indistinguishable mobilities and are all contained in the red ($i = 2$) carrier data of our MCT model and cannot be further separated with this method by merely increasing carrier count of the fitting.

In general, by following the $\mu_\mathrm{i}$ values it is easily possible to track the temperature trend of a particular carrier; the mobilities have a smooth, decreasing trend in temperature. An exception to this is the behavior of the red ($i = 2$) and blue ($i = 4$) carriers starting somewhere above 150 K in the datasets (see Fig. S2). There is a region where both the $\sigma_\mathrm{i}$ and $\mu_\mathrm{i}$ are close to each other, and above this temperature one cannot find a stable fit result without decreasing NC from 5 to 4. Considering the higher energy landscape of the electron bands in the band structure (Fig. 5 in main text), it is possible that this is a point where two electron carriers become inseparable by the MCT model, and must be represented as a single carrier. We have chosen to keep the $i = 4$ carrier at high temperatures, for a better continuity of $\mu_4$, but looking at e.g. devices D2 and D5 in Fig. S2, from the increase in $|\sigma_4|$ as well as the decrease in $\mu_4$, it is possible that the $i = 4$ carrier result is in fact the combined contribution of the two electron carriers at high temperature.

## V. BAND STRUCTURE CALCULATIONS

To compare the results of our MCT approach with the $ZrTe_5$ band structure, we performed DFT calculations to obtain the band structure, as a function of in-plane and out-of plane strain of the lattice. The optimized geometry and electronic properties of the crystal were obtained by the SIESTA implementation of DFT [3–6]. SIESTA employs norm-conserving pseudopotentials to account for the core electrons and linear combination of atomic orbitals to construct the valence states. The generalised gradient approximation of the exchange and the correlation functional was used with Perdew–Burke–Ernzerhof parametrisation [7] and the pseudopotentials optimised by Rivero *et al.* [8] with a double-$\zeta$ polarised basis set and a realspace grid defined with an equivalent energy cutoff of 350 Ry for the relaxation phase and 900 Ry for the single-point calculations. The Brillouin zone integration was sampled by a 30×30×18 Monkhorst–Pack $k$-grid for both the relaxation and the single-point calculations. [9] The geometry optimisations were performed until the forces were smaller than 0.1 eV $nm^{-1}$. The choice of pseudopotentials optimised by Rivero *et al.* ensures that both the obtained geometrical structures and the electronic band properties are reliable. After the successful self consistent cycles the necessary information was obtained by the sisl tool [10]. The spin orbit coupling was taken into account in the single point calculations.

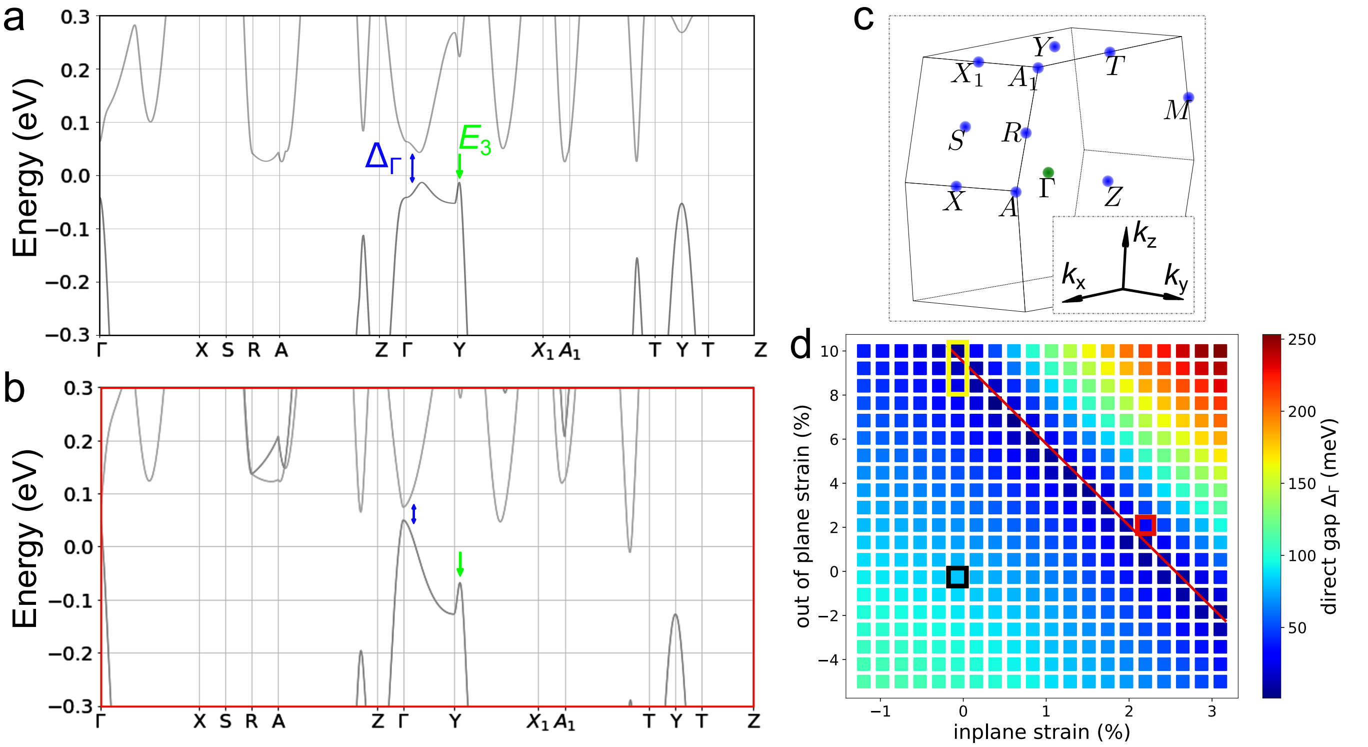


Figure S7. $ZrTe_5$ band structures calculated from DFT. (a) Default band structure using relaxed lattice parameters. The direct gap $\Delta_\Gamma$ and the band edge of the hole side-band associated with the MCT model carrier ($i = 3$), $E_3$, are denoted. (b) Band structure using approximately 2% isotropic strain. This is the band structure that matches the $\Delta_\Gamma$ and $E_3$ values obtained with the MCT model. (c) Brillouin zone and high symmetry points of $ZrTe_5$. (d) Colormap of the direct gap $\Delta_\Gamma$ as a function of uniform in-plane strain and out of plane strain. The STI-WTI phase transition occurs at $\Delta_\Gamma = 0$ (along the red line); the WTI phase is on the right side. The black square is the position of the band structure in (a) while the red square is that of (b). The yellow rectangle denotes a location where the appropriate $\Delta_\Gamma$ value is found using strain purely along the z-axis (vdW stacking).

The calculated relaxed lattice parameters are very close to the experimental lattice constants obtained from powder diffraction [11, 12], differing by about 1%. We notice that the band structure resulting from using these lattice parameters (Fig. S7 (a)), which results in a STI phase, does not match most of the results from our $n_{3D,i}(T)$ fitting. The size of the direct gap of the Dirac-like bands near Γ, $\Delta_\Gamma$, is significantly larger, the band edge energy of the green ($i = 3$) carrier, $E_3$, is at around the same energy as the Dirac-like holes ($i = 5$). The band structure is highly dependent on the lattice parameters, which can be seen on the strain-dependent colormap of $\Delta_\Gamma$ in Fig. S7 (d). The STI-WTI phase transition occurs where the gap fully closes. This defines a line on the colormap; however, the band

edge energy $E_3$ of the hole side band near Y also varies significantly along this direction. Therefore, the values of $\Delta_\Gamma$ and $E_3$ obtained from the MCT model can be used to find the appropriate position on the colormap.

We find that by applying an isotropic strain of around 2%, both the direct band gap as well as the position of the $i = 3$ pocket match it well (Fig. S7 (b)). This is the position in the $\Delta_\Gamma$ colormap where our MCT results best match the DFT in regards to both $\Delta_\Gamma$ and $E_3$. This position also results in a WTI phase. As mentioned in the main text, several experimental works provide various arguments as to why $ZrTe_5$ appears to exhibit WTI phase rather than the expected STI phase. This gives further support for our MCT results. We note here that the 2% strain is much too large to be accounted for by thermal expansion in the material (on the order of 0.2-0.4 % for 300 K). Therefore, the discrepancy between the relaxed lattice and the obtained band structure must be explained some other way. As mentioned in the main text, many other experiments also reveal such a discrepancy between DFT calculations and measured band structure details. Since the required strain modification of around 2% is comparable to the difference between DFT-based (relaxed) and experimental lattice parameters, and is also isotropic, it may be the case that the DFT method simply underestimates the unit cell size.

Alternatively, as described by Ref. [2], one can also think of applying merely out-of-plane strain (spacing of the layers in the vdW direction), and also reach a smaller direct band gap of the same value as obtained from our MCT model. However, in addition to a much larger value of the strain needed (up to 10% for also reaching the WTI phase), we also find that in this state the band edge energy $E_3$ is no longer consistent with the result of the MCT model. An interactive way to view the band structure calculation along the entire $\Delta_\Gamma$ colormap is available from Ref. [12] at `tajkov.ek-cer.hu/zrte5phasediagram/`.

Additionally we note that, as supported by the findings in Ref. [13] using flux-grown $ZrTe_5$ samples, the Fermi surface at the top of the valence band of Fig. S7 (a) in our calculations does indeed have a torus shape. However, in our devices, owing to the band shift and n-doping caused by the CVT growth method, the chemical potential at 2 K is closer to 100 meV on Fig. S7 (b). Consequently, our SdHO measurements reveal the presence of two distinct electron pockets, as detailed in the SdHO section.


[1] F. Tang, Y. Ren, P. Wang, R. Zhong, J. Schneeloch, S. A. Yang, K. Yang, P. A. Lee, G. Gu, Z. Qiao, and L. Zhang, Three-dimensional quantum Hall effect and metal–insulator transition in $ZrTe_5$, Nature **569**, 537–541 (2019).

[2] Y. Zhang, C. Wang, L. Yu, G. Liu, A. Liang, J. Huang, S. Nie, X. Sun, Y. Zhang, B. Shen, *et al.*, Electronic evidence of temperature-induced Lifshitz transition and topological nature in $ZrTe_5$, Nature Communications **8**, 15512 (2017).

[3] E. Artacho, E. Anglada, O. Diéguez, J. D. Gale, A. García, J. Junquera, R. M. Martin, P. Ordejón, J. M. Pruneda, D. Sánchez-Portal, and J. M. Soler, The SIESTA method; developments and applicability, Journal of Physics: Condensed Matter **20**, 064208 (2008).

[4] J. M. Soler, E. Artacho, J. D. Gale, A. García, J. Junquera, P. Ordejón, and D. Sánchez-Portal, The SIESTA method for ab initio order-N materials simulation, Journal of Physics: Condensed Matter **14**, 2745 (2002).

[5] A. García, N. Papior, A. Akhtar, E. Artacho, V. Blum, E. Bosoni, P. Brandimarte, M. Brandbyge, J. I. Cerdá, F. Corsetti, *et al.*, Siesta: Recent developments and applications, The Journal of chemical physics **152**, 204108 (2020).

[6] L. Fernández-Seivane, M. A. Oliveira, S. Sanvito, and J. Ferrer, On-site approximation for spin–orbit coupling in linear combination of atomic orbitals density functional methods, Journal of Physics: Condensed Matter **18**, 7999 (2006).

[7] J. P. Perdew, K. Burke, and M. Ernzerhof, Generalized gradient approximation made simple, Physical Review Letters **77**, 3865 (1996).

[8] P. Rivero, V. M. García-Suárez, D. Pereñiguez, K. Utt, Y. Yang, L. Bellaiche, K. Park, J. Ferrer, and S. Barraza-Lopez, Systematic pseudopotentials from reference eigenvalue sets for DFT calculations, Computational Materials Science **98**, 372 (2015).

[9] H. J. Monkhorst and J. D. Pack, Special points for Brillouin-zone integrations, Physical Review B **13**, 5188 (1976).

[10] N. Papior, sisl: v0.11.0 (2021).

[11] H. Fjellvåg and A. Kjekshus, Structural properties of $ZrTe_5$ and $HfTe_5$ as seen by powder diffraction, Solid State Communications **60**, 91 (1986).

[12] Z. Tajkov, D. Nagy, K. Kandrai, J. Koltai, L. Oroszlány, P. Süle, Z. E. Horváth, P. Vancsó, L. Tapasztó, and P. Nemes-Incze, Revealing the topological phase diagram of $ZrTe_5$ using the complex strain fields of microbubbles, npj Computational Materials **8**, 177 (2022).

[13] Y. Wang, H. F. Legg, T. Bömerich, J. Park, S. Biesenkamp, A. A. Taskin, M. Braden, A. Rosch, and Y. Ando, Gigantic Magnetochiral Anisotropy in the Topological Semimetal $ZrTe_5$, Phys. Rev. Lett. **128**, 176602 (2022).
